# Supplementary material for: Bounds on half graph orders in powers of sparse graphs
Source: arXiv:2103.06218 source file (2021-03-10)
Supplement: Supplementary file 3 [file pw-appendix-join-c.tex]

\documentclass{standalone}

\usepackage{amssymb}
\usepackage{tikz}
\usetikzlibrary{calc,positioning}
\usepackage{color, colortbl}

\begin{document}

\begin{tikzpicture}[auto, every loop/.style={},
                    top/.style={circle,minimum size=0.4cm,inner sep=0pt,draw},
                    smol/.style={circle,minimum size=0.12cm,inner sep=0pt,draw, gray}]

  \node [top] (r) at (0, 1) {$r$};
  \node [top] (b) at (0, -0.2) {$b_i$};
  \foreach \name/\x in {2/-0.5, 3/0, 4/0.5, 5/1} {
    \foreach \i/\y in {1/-1, 2/-1.5, 3/-2, 4/-2.5, 5/-3, 6/-3.5} {
      \node [smol] (m\name\i) at (\x, \y) {};
    };
    \foreach \i [count=\yi] in {2,...,6} {
      \draw [gray] (m\name\yi) -- (m\name\i);
    };
    \draw [gray] (b) -- (m\name 1);
  };
  \foreach \i/\y in {1/-1, 2/-1.5, 3/-2, 4/-2.5} {
    \node [smol, black] (m1\i) at (-1, \y) {};
  }
  \foreach \i [count=\yi] in {2,...,4} {
    \draw (m1\yi) -- (m1\i);
  };
  \draw (b) -- (m11);
  \draw (m14) to [bend left=20] (-1.6, -1.2) to [bend left=38] (r);
\end{tikzpicture}

\end{document}
